# Supplementary material for: Searching for Optimal Runtime Assurance via Reachability and Reinforcement Learning
Source: arXiv:2310.04288 source file (2023-10-06)
Supplement: Supplementary file 1 [file appendix.tex]

\section{Agent models}
\label{app:models}

The dynamics for $\acc$ are given by
\begin{gather}
    \nonumber \dot{x} = v \\
    \dot{v} = a^c
\end{gather}
where the state is given by $q = [x \ v]^{\top}$ and the input is given by $u = a^c$.
The dynamics for $\dubins$ are given by 
\begin{gather}
    \nonumber \dot{x} = v \cos{\yaw} \\
    \nonumber \dot{y} = v \sin{\yaw} \\
    \nonumber \dot{\yaw} = \yawInput \\
    \dot{v} = a^c
\end{gather}
where the state is given by $q = [x \ y \ \yaw \ v]^{\top}$ and the input is given by $u = [\yawInput \ a^c]^{\top}$.
The dynamics for $\air$ are given by
\begin{gather}
    \nonumber \dot{x} = v \cos{\yaw} \cos{\pitch} \\
    \nonumber \dot{y} = v \sin{\yaw} \cos{\pitch} \\
    \nonumber \dot{z} = v \sin{\pitch} \\
    \nonumber \dot{\yaw} = \yawInput \\
    \nonumber \dot{\pitch} = \pitchInput \\
    \dot{v} = a^c
\end{gather}
where the state is given by $q = [x \ y \ z \ \yaw \ \pitch \ v]^{\top}$ and the input is given by $u = [\yawInput \ \pitchInput \ a^c]^{\top}$.

\section{Controllers}
\label{app:controllers}
\kristina{Describe the controllers in this section}
